# Supplementary material for: Faster Game Solving via Predictive Blackwell Approachability: Connecting Regret Matching and Mirror Descent
Source: arXiv:2007.14358 source file (2021-03-08)
Supplement: Supplementary file 1 [file appendix_w_regret.tex]

\section{$w$-Regret}

\begin{definition}
	Let $w^1,\dots,w^T$ be a sequence of weakly increasing positive reals. The
	$w$-regret incurred by the decision maker is defined as 
	\[
		R_w^T(\hat{\vec{x}}) \defeq \sum_{t=1}^T w^t \langle \vec{\ell}^t, \vec{x}^t - \hat{\vec{x}}\rangle.
	\]
\end{definition}

\begin{proposition}
	At all times $T$, OMD guarantees that
	\[
		R_w^T(\hat{\vec{x}}) \le w^T\mleft( \frac{\div{\hat{\vec{x}}}{\vec{z}^0}}{\eta} + \eta \sum_{t=1}^T \|\vec{\ell}^t - \vec{m}^t\|_*^2 - \frac{1}{8\eta}\sum_{t=1}^{T-1} \|\vec{x}^{t+1}-\vec{x}^t\|^2\mright) + \frac{w^T}{\eta} \max_{t=1}^T \div{\hat{\vec{x}}}{\vec{x}^t}.
	\]
\end{proposition}

\begin{proposition}
	\[
		\min_{\hat{\vec{s}} \in C} \mleft\| \hat{\vec{s}} - \frac{1}{\sum w^t}\sum_{t=1}^T w^t\cdot \vec{u}(\vec{x}^t,\vec{y}^t)\mright\|_2 \le \frac{1}{\sum w^t} \max_{\hat{x}\in\cK} R_w^T(\hat{\vec{x}}).
	\]
\end{proposition}

So, in order to retain guarantees for linear or quadratic averaging, it is
enough to show that the right-hand side is $O(1/\sqrt{T})$. 

\begin{proposition}
	At all times $T$, 
\end{proposition}
